# Supplementary material for: Fitting Prediction Rule Ensembles to Psychological Research Data: An Introduction and Tutorial
Source: arXiv:1907.05302 ancillary file (2023-09-29)
Supplement: Supplementary file 1 [file R_scripts_and_instructions.pdf]

# Replication Scripts for “Fitting Prediction Rule Ensembles to Psychological Research Data: An Introduction and Tutorial”

This document provides a manual on how to fit prediction rule ensembles (PREs) as in the examples from the main paper. In what follows, the code and results of fitting PREs using **R** package **pre** is provided, intermingled with comments and explanations. Some experience in **R** is recommended (e.g., loading data, fitting a regression model using function `lm()`). Readers who have not used **R** before are advised to first follow the (very) short introduction of Torfs & Brauer (2014).

This manual is structured as follows: In the first three sections, we replicate the analyses of each of the three examples from the main paper: predicting chronic depression (Example 1), academic achievement (Example 2) and substance use (Example 3). In the fourth and last section, we explain the main parameters that control the model-fitting process, and how these affect computation time, and complexity and predictive accuracy of the final ensemble. Because the parameter settings that yield optimal predictive accuracy will often depend on the data problem at hand, the last section also shows how optimal parameter values can be selected using cross validation.

Because we do not own the datasets analyzed in the main paper, in this tutorial we replicate the analyses on artificially generated datasets, which are also provided in the Supplementary Material. These datasets were generated so that the univariate distributions are the same as those in the original datasets, but the inter-correlations between variables are different. Therefore, results will differ from those presented in the main paper and do not represent accurate empirical results.

The results in this document have been obtained using **R** (R Core Team, 2019, version 3.6.1) using packages **pre** (Fokkema, n.d., version 0.7.2), **partykit** (Hothorn & Zeileis, 2015, version 1.2–5), **glmnet** (Friedman, Hastie, & Tibshirani, 2010, version 3.0–1) and **caret** (Kuhn, 2008, version 6.0–84).

## Installing and loading the package

Before we start the analyses, we first install package **pre** by typing in **R**:

```
install.packages("pre")
```

The package needs to be installed only once. Once it has been installed, we can load the package into **R** by

typing:

```
library("pre")
```

## Example 1: Predicting Chronic Depression

We replicate the analyses on predicting chronic depression using the `depression.txt` file, which is available in the online Supplementary Material. After downloading the file, it should be made available in **R**'s current working directory, which can be accomplished in one of two ways: We can request the location of the current working directory by typing:

```
getwd()
```

and then place the `depression.txt` file in that location. Alternatively, we can set the working directory to the location of the `depression.txt` file using function `setwd()`.

```
setwd("path_to_folder_containing_file")
```

We can then load the data into **R** by typing:

```
depression <- read.table("depression.txt")
```

We can check the number of columns (variables) and rows (observations) of the dataset by typing:

```
dim(depression)
```

```
[1] 682 21
```

To get an overview of the types of variables in the dataset, we use function `head` to print the first six rows:

```
head(depression)
```

|   | dep |            | disType  | Sexe   | Age | edu_yrs | IDS | BAI | FQ | LCImax | pedigree | alcohol  |
|---|-----|------------|----------|--------|-----|---------|-----|-----|----|--------|----------|----------|
| 1 | No  | comorbid   | disorder | female | 43  | 15      | 18  | 14  | 6  | 0.093  | Yes      | Positive |
| 2 | Yes | depressive | disorder | female | 38  | 15      | 14  | 15  | 0  | 0.367  | Yes      | Positive |
| 3 | No  | depressive | disorder | female | 26  | 9       | 22  | 6   | 20 | 1.000  | Yes      | Positive |
| 4 | Yes | depressive | disorder | female | 30  | 11      | 8   | 8   | 11 | 1.000  | No       | Positive |
| 5 | Yes | comorbid   | disorder | female | 36  | 12      | 13  | 15  | 0  | 0.583  | Yes      | Positive |
| 6 | No  | comorbid   | disorder | female | 40  | 15      | 17  | 27  | 7  | 0.912  | Yes      | Positive |

  

|   | TypeDep     | SocPhob | GAD      | Panic    | Ago      | A0       | RemDis |     |
|---|-------------|---------|----------|----------|----------|----------|--------|-----|
| 1 | First onset | MDD     | Negative | Negative | Negative | Negative | 16     | No  |
| 2 | Recurrent   | MDD     | Negative | Negative | Negative | Negative | 36     | Yes |
| 3 | First onset | MDD     | Negative | Negative | Positive | Negative | 12     | No  |
| 4 | Recurrent   | MDD     | Negative | Negative | Negative | Negative | 10     | No  |
| 5 | Recurrent   | MDD     | Positive | Negative | Negative | Negative | 12     | No  |

|   |                          |          |            |          |          |    |    |
|---|--------------------------|----------|------------|----------|----------|----|----|
| 6 | Recurrent MDD            | Negative | Negative   | Positive | Negative | 51 | No |
|   | sample                   | ADuse    | PsychTreat |          |          |    |    |
| 1 | Primary care             | Yes      | Yes        |          |          |    |    |
| 2 | Spec. mental health care | Yes      | Yes        |          |          |    |    |
| 3 | Primary care             | Yes      | No         |          |          |    |    |
| 4 | General population       | No       | No         |          |          |    |    |
| 5 | Spec. mental health care | No       | No         |          |          |    |    |
| 6 | Spec. mental health care | No       | Yes        |          |          |    |    |

The first variable in the dataset (`dep`) is the response variable; it is an indicator for whether subjects still meet the criteria of depression two years after baseline (i.e., a chronic depression trajectory). The other variables are potential predictors measured at baseline and are described in more detail in the main paper.

Fitting a PRE requires random sampling of the training observations for generating rules. We therefore first have to set the state of **R**'s random number generator, which will allow for exact replication of the results at a later time:

```
set.seed(1)
```

We will now fit the ensemble using function `pre()`. The first argument of this function specifies the model to be fitted: the response and potential predictor variables, separated by a tilde (`~`). Here we use the dot (`.`) as short-hand notation for regressing the specified response (`dep`) on all remaining variables in the dataset. Because the response is a binary factor, we also specify `family = "binomial"`:

```
depression.ens <- pre(dep ~ ., data = depression, family = "binomial")
```

Alternatively, if we want to specify only a subset of the variables as possible predictors, we would specify the model by enumerating the subset of predictors using the `+` sign, for example:

```
dep ~ LCImax + IDS + PsychTreat
```

We can obtain a summary of the fitted ensemble as follows:

```
summary(depression.ens)
```

Final ensemble with cv error within 1se of minimum:

```
lambda = 0.02027569
number of terms = 11
mean cv error (se) = 1.306071 (0.0105627)
```

The results indicate the criterion used for selecting the optimal value of the penalty parameter  $\lambda$ : the value

yielding a cross-validated prediction error within one standard error of the minimum. Furthermore, the results indicate that 11 terms were selected in the final PRE. Also, the cross-validated error of the selected  $\lambda$  value is reported, but it should be noted that this estimate likely provides an overly optimistic value of the expected prediction error, as it was calculated using the same data as was used to generate the rules. Later, we will use function `cvpre()` to obtain a more realistic estimate of future prediction error.

To further inspect the ensemble, we can print it as follows:

```
depression.ens
```

```
(Intercept) -0.142840437      1
rule83      0.465783036    LCImax > 0.273 & IDS > 12
rule74     -0.364372821      IDS <= 16 & AO > 16
rule58      0.172394168      IDS > 16 & AO > 19
rule4      -0.129596029      IDS <= 16 & Age > 45
rule87      0.120583987    Age <= 51 & LCImax > 0.327
rule53      0.108963183      IDS > 11 & LCImax > 0.265
rule71      0.075324759      LCImax > 0.298 & IDS > 10
rule50      0.020192727      LCImax > 0.339 & IDS > 11
rule56     -0.014485365      IDS <= 16 & Age > 36
rule41      0.010042401      IDS > 13 & LCImax > 0.273
rule14     -0.005711446    IDS <= 16 & LCImax <= 0.847
```

Alternatively, we could have typed `print(depression.ens)`, which would have yielded the exact same result. The printed results provide a description of the rules and/or linear terms included in the final ensemble, with their respective coefficients. Note that in this case, no linear terms were selected, as the column `rule` only contains (numbered) rules. If linear terms were selected, this column would also show the names of the selected predictor variables.

The rules are ordered by the absolute value of their coefficients. The coefficient of rule `rule83` (`LCImax > 0.273 & IDS > 12`) indicates that meeting the criteria of this rule increases the log odds of a chronic depression by about 0.47. Note that all rules involve only four variables: `LCImax` (proportion of time in which symptoms of anxiety or depression were present in the four years prior to baseline), `IDS` (psychological test score reflecting severity of depressive symptoms), `AO` (age of disorder onset) and `Age` (in years); the remaining variables in the dataset thus appear unimportant for predicting chronic depression.

To generate predictions for new observations, the contributions of each rule and linear term in the final ensemble need to be computed and summed. Predictions can be computed using the `predict` method, which

requires the user to supply the fitted ensemble and the `newdata` argument, which should supply a dataframe of observations for which predictions will be computed. If the `newdata` argument is not specified, predictions for the original training observations are returned. Here, we request predictions for four of the training observations. By default, the `predict` method returns predictions on the scale of the linear predictors. Through specifying `type = "response"`, we obtain the predicted probabilities:

```
predict(depression.ens, newdata = depression[c(1, 3, 5, 7),], type = "response")
```

```
      1      3      5      7
0.4643505 0.6588221 0.6552722 0.3663186
```

Observations 1 and 7 obtained somewhat lower predicted probabilities, while observations 3 and 5 obtained somewhat higher predicted probabilities. We can use function `explain()` to obtain an explanation of these predictions:

```
expl <- explain(depression.ens, newdata = depression[c(1, 3, 5, 7),])
```

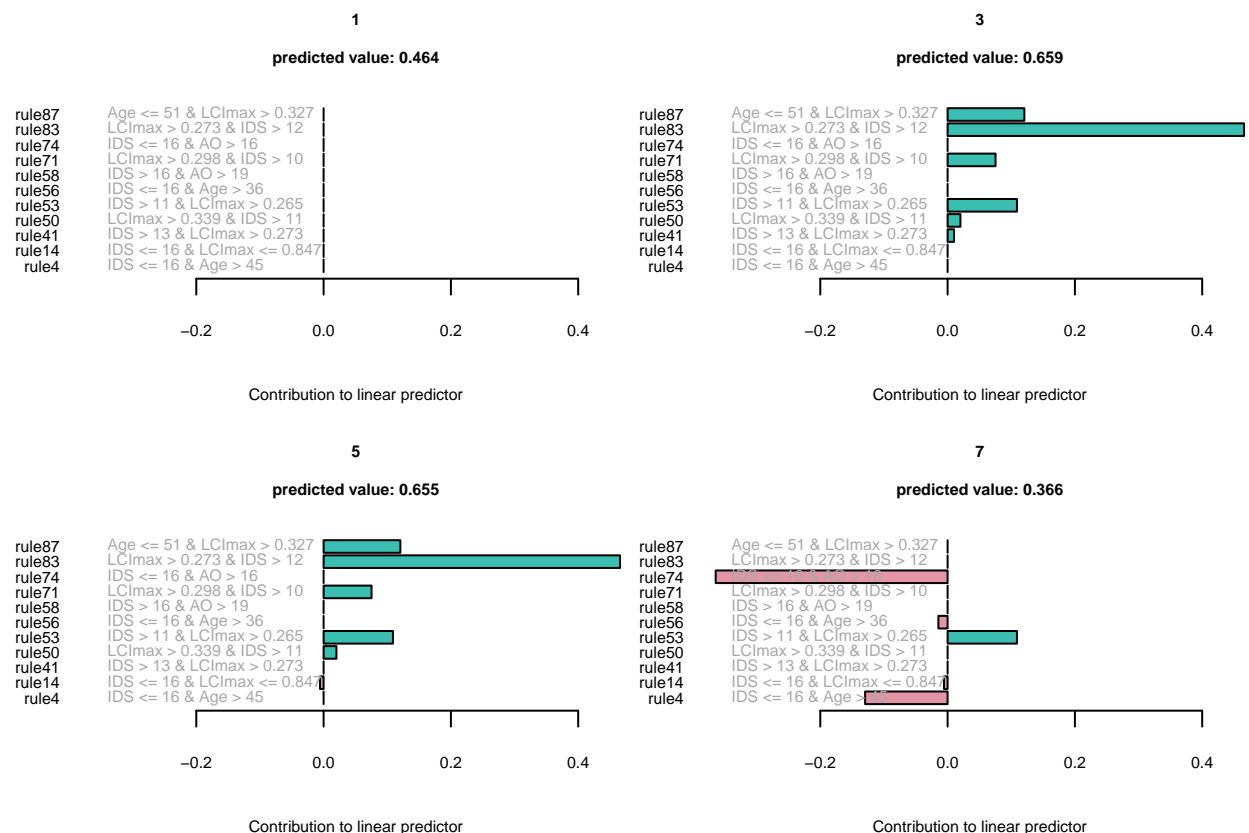

Numerical results are saved in `expl$predictors` (which provides the values of the predictor variables) and `expl$contribution` (which provides the contribution of each term to the individual predictions, as plotted above).

The plotted results show the predicted probabilities, and the contributions of the terms in the final ensemble to the observation-level predictions. Green bars reflect contributions to the predicted value of rules with positive coefficients, while red bars represent contributions of rules with negative coefficients. The absence of a vertical green or red bar indicates that the observation did not meet the conditions of that rule. The rules are ordered from top to bottom in ascending order of global importance. Note that the contributions are on the scale of the linear predictor, thus reflecting the increase in log odds of belonging to the target class (i.e., having a chronic depression trajectory).

The first plot reveals that observation 1 did not meet the conditions of any rule. The predicted probability for this observation is therefore based on the value of the intercept only:  $\frac{e^{-0.143}}{1+e^{-0.143}} = 0.464$ . Observations 3 and 5 obtained a higher predicted probability, because they meet the conditions of several rules with positive coefficients. Observation 7 meets the conditions of several rules with negative coefficients, resulting in a lower predicted probability.

To obtain an overview of the importances of baselearners (rules and/or linear terms) and predictor variables, we use the `importance()` function, which by default creates a plot of the variable importances:

```
depression.imp <- importance(depression.ens)
```

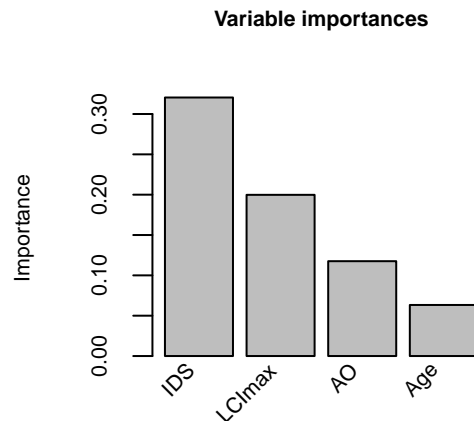

The plot indicates that the ensemble included only four of the potential predictor variables, which we also observed through inspecting the rules. The remaining variables were not part of any rule or linear term in the final ensemble and thus obtained importances of 0. In addition to plotting the predictor variable importances, function `importance()` invisibly returns a list of variable and baselearner importances, which we have assigned to the `depression.imp` object with the code above. We can access the numeric values of

these importances as follows:

```
depression.imp$varimps
```

```
varname      imp
1      IDS 0.32046825
2    LCImax 0.19981898
3       AO 0.11758793
4      Age 0.06330385
```

```
depression.imp$baseimps
```

|    | rule   | description                 | imp         | coefficient  | sd        |
|----|--------|-----------------------------|-------------|--------------|-----------|
| 1  | rule83 | LCImax > 0.273 & IDS > 12   | 0.229547451 | 0.465783036  | 0.4928205 |
| 2  | rule74 | IDS <= 16 & AO > 16         | 0.180269504 | -0.364372821 | 0.4947392 |
| 3  | rule87 | Age <= 51 & LCImax > 0.327  | 0.060242513 | 0.120583987  | 0.4995897 |
| 4  | rule4  | IDS <= 16 & Age > 45        | 0.059128453 | -0.129596029 | 0.4562520 |
| 5  | rule58 | IDS > 16 & AO > 19          | 0.054906353 | 0.172394168  | 0.3184931 |
| 6  | rule53 | IDS > 11 & LCImax > 0.265   | 0.054515717 | 0.108963183  | 0.5003132 |
| 7  | rule71 | LCImax > 0.298 & IDS > 10   | 0.037689859 | 0.075324759  | 0.5003648 |
| 8  | rule50 | LCImax > 0.339 & IDS > 11   | 0.009976282 | 0.020192727  | 0.4940532 |
| 9  | rule56 | IDS <= 16 & Age > 36        | 0.007236739 | -0.014485365 | 0.4995897 |
| 10 | rule41 | IDS > 13 & LCImax > 0.273   | 0.004817301 | 0.010042401  | 0.4796961 |
| 11 | rule14 | IDS <= 16 & LCImax <= 0.847 | 0.002848846 | -0.005711446 | 0.4987960 |

We can obtain univariate partial dependence plots using the `singleplot()` function. We use the `varname` argument to specify the name of the predictor variable for which we want to plot the partial dependence:

```
singleplot(depression.ens, varname = "IDS")
singleplot(depression.ens, varname = "LCImax")
```

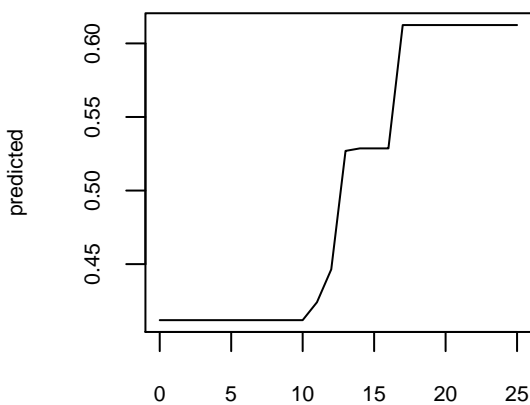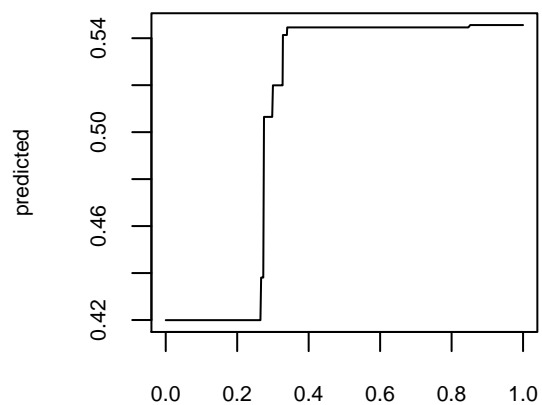

The univariate partial dependence plots reveal a monotonously increasing effect of both IDS and LCImax on

the predicted probability of a chronic trajectory.

We can obtain a bivariate partial dependence plot using the `pairplot()` function. This function requires package **akima** to be installed; if the package is not installed yet, we first need to install it as follows:

```
install.packages("akima")
```

Then, we call function `pairplot()` and specify the names of two predictor variables with the `varnames` argument:

```
pairplot(depression.ens, varnames = c("IDS", "LCImax"))
```

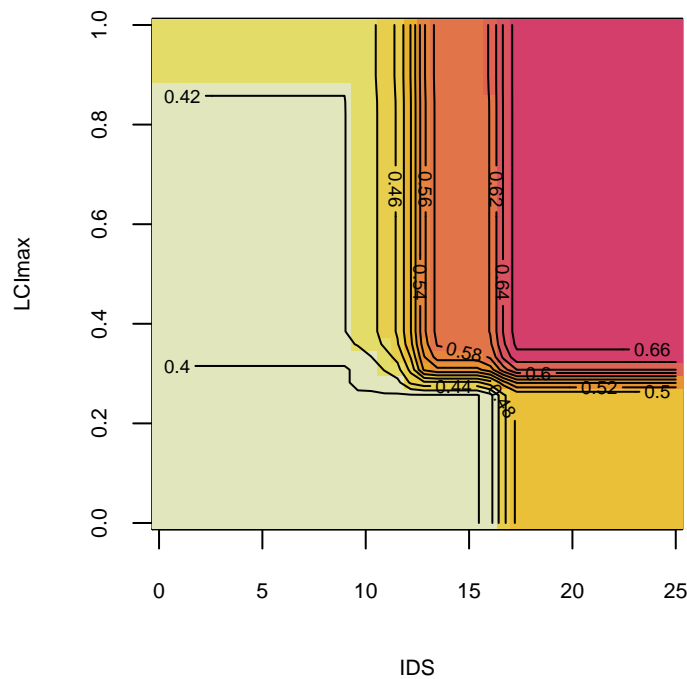

In the bivariate partial dependence plot, the yellow (lighter) areas correspond to lower predicted probabilities, while the red (darker) areas correspond to higher predicted probabilities. The contour lines depict areas with similar predicted values. Like the univariate plots, the bivariate partial dependence plot also reveals that the predicted probability of a chronic trajectory increases with increasing values of `IDS` and/or `LCImax`.

To obtain a realistic estimate of the fitted ensemble's prediction error on future observations, we use function `cvpre()`. This function estimates the expected predictive accuracy using  $k$ -fold cross validation. It first separates the original training data into  $k$  (approximately) equally sized test samples. Each of the  $k$  test

samples is then used to assess predictive accuracy of a model fitted on the remaining training observations (i.e., observations that are not in the current test sample). This model is fitted using the same settings as those used for fitting the original model (i.e., `depression.ens`, which was fitted using the default settings).

By default, `cvpre()` performs ten-fold cross validation, but a different number of folds can be specified through argument `k`. Random sampling is used to assign observations to folds, so the results depend on the random seed we have set above.

```
cv.depression <- cvpre(depression.ens)
```

```
$SEL
```

```
      SEL      se
0.240917416 0.003293254
```

```
$AEL
```

```
      AEL      se
0.483243007 0.003294995
```

```
$MCR
```

```
[1] 0.3944282
```

```
$table
```

```
      observed
predicted      No      Yes
No  0.3240469 0.2243402
Yes 0.1700880 0.2815249
```

The printed results show the squared error loss (**SEL**) and absolute error loss (**AEL**) with their respective standard errors, the misclassification rate (**MCR**) and a confusion matrix (**table**). These are also stored in `cv.depression$accuracy` for possible later use. The MCR indicates that (100-39.44=)60.56 % of observations were correctly classified.

The cross-validated predictions for every observation can be extracted from `cv.depression$cvpreds`. This allows for calculation of alternative accuracy estimates. For example, we may want to calculate the correlation between the predicted probability of belonging to the target class and the observed class membership (a.k.a. the point-biserial correlation):

```
cor(cv.depression$cvpreds, as.numeric(depression$dep))
```

```
      [,1]
[1,] 0.1909607
```

## Example 2: Predicting Academic Achievement

Using the data contained in the `achievement.txt` file, we will replicate the analyses on predicting academic achievement. This example featured a multivariate response variable, as well as non-negativity constraints in order to obtain only positive coefficients for rules and linear terms. We first read in the data as follows:

```
achievement <- read.table("achievement.txt")
dim(achievement)
```

```
[1] 638 11
```

```
head(achievement)
```

|   | Gender | Nationality | Age | Online_test        | Test_Language | RawScore_English |
|---|--------|-------------|-----|--------------------|---------------|------------------|
| 1 | female | Dutch       | 20  | present at testday | English       | 15               |
| 2 | female | German      | 20  | present at testday | Dutch         | 17               |
| 3 | male   | Dutch       | 21  | present at testday | Dutch         | 18               |
| 4 | male   | EU          | 19  | present at testday | English       | 20               |
| 5 | male   | German      | 18  | present at testday | English       | 17               |
| 6 | female | German      | 21  | online             | Dutch         | 15               |

  

|   | RawScore_Math | RawScore_Psychology | Program | MeanFYG | Credits |
|---|---------------|---------------------|---------|---------|---------|
| 1 | 18            | 28                  | Dutch   | 6.5     | 55.0    |
| 2 | 26            | 21                  | Dutch   | 5.3     | 17.5    |
| 3 | 8             | 29                  | English | 6.9     | 8.0     |
| 4 | 22            | 30                  | English | 4.2     | 60.0    |
| 5 | 12            | 37                  | English | 6.1     | 50.0    |
| 6 | 18            | 37                  | English | 7.2     | 55.0    |

The dataset comprises 638 observations on 11 variables, of which the last two (**MeanFYG** and **Credits**) are the response variables, reflecting the average grade for the first-year psychology courses and the total number of study credits obtained in the first year. The other variables are potential predictor variables and are described in the main paper.

To specify the model formula for a multivariate response, we will specify **Credits** and **MeanFYG** before the tilde, separated by the plus sign. Furthermore, we specify a multivariate Gaussian response distribution through the **family** argument.

To apply the non-negativity constraint, we specify a lower limit of 0 for the estimated penalized coefficients through the **lower.limits** argument. In addition, we set the **removecomplements** argument to **FALSE**. By default, when the initial ensemble contains rules that are perfectly (negatively or positively) correlated, **pre()** retains only one of these rules. This likely reduces computation time and complexity of the final ensemble, but does not affect predictive accuracy of the final ensemble. When a (non-)negativity constraint is applied,

however, removal of negatively correlated rules can negatively affect predictive accuracy, and should therefore be suppressed by specifying the `removecomplements` argument:

```
set.seed(2)
achievement.ens <- pre(Credits + MeanFYG ~ ., data = achievement,
                      family = "mgussian", lower.limits = 0,
                      removecomplements = FALSE)
achievement.ens
```

Final ensemble with cv error within 1se of minimum:

```
lambda = 1.395596
number of terms = 9
mean cv error (se) = 207.116 (17.40264)
```

cv error type : Mean-Squared Error

| rule        | coefficient.Credits | coefficient.MeanFYG |
|-------------|---------------------|---------------------|
| (Intercept) | 29.1671545097       | 5.45409977827       |
| rule3       | 7.3987510599        | 0.50084345213       |
| rule32      | 6.5846584758        | 0.45584196175       |
| rule17      | 3.8300890713        | 0.23468305860       |
| rule14      | 3.5459869453        | 0.23182026310       |
| rule145     | 1.5636003680        | 0.09283659879       |
| rule96      | 1.1527442881        | 0.08932119664       |
| rule9       | 1.2693025569        | 0.08173663400       |
| rule126     | 1.0417745521        | 0.05570609097       |
| rule127     | 0.0006591047        | 0.00003359027       |

| rule        | description                                                                                          |
|-------------|------------------------------------------------------------------------------------------------------|
| (Intercept) | 1                                                                                                    |
| rule3       | RawScore_Psychology > 24 & Nationality %in% c("Dutch", "German")                                     |
| rule32      | RawScore_Psychology > 24 & RawScore_Math > 12                                                        |
| rule17      | RawScore_Psychology > 25 & Nationality %in% c("Dutch", "German")                                     |
| rule14      | RawScore_Psychology > 24 & Nationality %in% c("Dutch", "German") & RawScore_Math > 8                 |
| rule145     | RawScore_Psychology > 24 & Nationality %in% c("Dutch", "German", "Non-EU") & Gender %in% c("female") |
| rule96      | RawScore_Psychology > 24 & Nationality %in% c("Dutch", "EU", "German") & RawScore_Math > 13          |
| rule9       | RawScore_Psychology > 24 & Nationality %in% c("Dutch", "German") & Gender %in% c("female")           |
| rule126     | RawScore_Math > 8 & RawScore_Psychology > 25                                                         |
| rule127     | RawScore_Math > 8 & RawScore_Psychology > 25 & Nationality %in% c("Dutch", "German", "Non-EU")       |

Table 1: Rule descriptions of the ensemble for predicting academic achievement.

The final ensemble for predicting academic achievement comprises 9 rules. Note that each rule (or linear term) obtained two estimated coefficients, one for each response variable. Because the rule descriptions are rather long, they are omitted from the verbatim output here and presented in Table 1. Table 1 shows that many rules involve the scores on the psychology and math admission tests, and nationality. Gender occurs in some of the rules.

To further interpret the ensemble, we request standardized variable importances, which allow for comparing the importance of rules, linear terms and predictor variables between response variables with different scales:

```
achievement.imp <- importance(achievement.ens, standardize = TRUE)
```

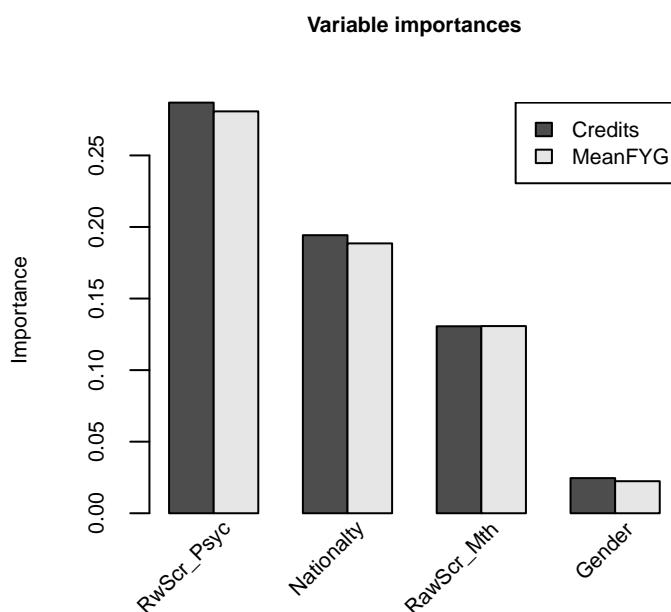

The importances for the two response variables appear quite similar. As we already observed in the rule descriptions (Table 1), only four of the potential predictor variables contribute to the predictions of the response variables.

Using function `cvpre()`, we can obtain an estimate of future prediction error:

```
cv.achievement <- cvpre(achievement.ens)
```

```
$MSE
      MSE      se
Credits 202.8624086 10.11439502
MeanFYG  0.9447364  0.05403603
```

```

$MAE
      MAE      se
Credits 10.5387861 0.26842818
MeanFYG  0.7270352 0.01807355

```

Mean squared error (MSE) and mean absolute error (MAE) are printed and also saved in `cv.achievement$accuracy`. The cross-validated predictions are saved in `cv.achievement$cvpreds` and can be used to calculate alternative indices of accuracy, like the correlation between observed and predicted values:

```
cor(cv.achievement$cvpreds[ , "Credits"], achievement$Credits)
```

```
[1] 0.6918321
```

```
cor(cv.achievement$cvpreds[ , "MeanFYG"], achievement$MeanFYG)
```

```
[1] 0.6853558
```

## Example 3: Predicting Substance Use

We replicate the analyses of the third example, prediction of substance use in the last week of a randomized clinical trial, using the `drug_usage` data:

```
drug_usage <- read.table("drug_usage.txt")
dim(drug_usage)
```

```
[1] 478  57
```

```
names(drug_usage)
```

```

[1] "DSPRIMAR"      "trt"           "AGEYRS"        "DEGENDER"      "SCLVLEDU"
[6] "SCMARITA"      "SCEMPLOY"      "SCLIVING"      "QOHLTHST.TO"   "QOMOBIL.TO"
[11] "QOSLFCAR.TO"   "QOACTIVE.TO"   "QOPAIN.TO"     "QOANXDEP.TO"   "BSFNTDIZ.TO"
[16] "BSNOINT.TO"    "BSNERVOS.TO"   "BSPAINHR.TO"   "BSLONELY.TO"   "BSTENSE.TO"
[21] "BSNAUSE.TO"    "BSBLUE.TO"     "BSSCARED.TO"   "BSBREATH.TO"   "BSWORTH.TO"
[26] "BSTERRO.TO"    "BSNUMB.TO"     "BSHOPELS.TO"   "BSRESTLS.TO"   "BSWEAK.TO"
[31] "BSENDLIF.TO"   "BSFEARFL.TO"   "CSPHYACT.TO"   "CSAVOID.TO"    "CSFEELGD.TO"
[36] "CSREMOVE.TO"   "CSNOOFFR.TO"   "CSOTHTHG.TO"   "CSOVRCOM.TO"   "CSSOMELS.TO"
[41] "CSTRYHRD.TO"   "CSLEAVE.TO"    "CSSOCIAL.TO"   "CSDOGOOD.TO"   "CSPHYREA.TO"
[46] "CSCALM.TO"     "CSSAYNO.TO"    "CSPOSOUT.TO"   "CSACCOMP.TO"   "CSDIFFIC.TO"
[51] "CSDEAL.TO"     "CSWAIT.TO"     "CSSTAYAW.TO"   "CSSTONEG.TO"   "CSEMOTIO.TO"
[56] "week1"         "week12"

```

The dataset consists of 478 observations on 57 variables. The last variable, `week12`, is the response, reflecting the number of days drugs or alcohol were used in the last (12th) week of substance use treatment. The remaining

variables are possible predictors, assessed at the start of treatment: socio-demographic characteristics, items of a quality of life measure (starting with QO), a brief mental-health symptom inventory (starting with BS) and a coping scale (starting with CS). The variables are described in more detail in the main paper.

As the response variable reflects a count of events, we use the `family` argument to specify a Poisson distribution. Also, we include the treatment indicator as a confirmatory rule, as earlier studies indicated that TES (treatment with the therapeutic education system) resulted in lower average substance abuse rates, compared to TAU (treatment as usual). We specify the confirmatory rule with the `confirmatory` argument, so its estimated coefficient will not be penalized (i.e., not shrunk towards zero):

```
set.seed(3)
drug_usage.ens <- pre(week12 ~ ., data = drug_usage, family = "poisson",
                     confirmatory = "trt %in% 'TES'")
```

```
drug_usage.ens
```

Final ensemble with cv error within 1se of minimum:

```
lambda = 0.1346009
number of terms = 7
mean cv error (se) = 2.21122 (0.11118)
```

cv error type : Poisson Deviance

|  | rule           | coefficient |                               | description    |
|--|----------------|-------------|-------------------------------|----------------|
|  | (Intercept)    | 0.95406494  |                               | 1              |
|  | trt %in% 'TES' | -0.68455326 |                               | trt %in% 'TES' |
|  | rule3          | -0.40324259 | week1 <= 0 & BSSCARED.T0 <= 1 |                |
|  | rule15         | -0.31325359 | week1 <= 0 & BSTENSE.T0 <= 3  |                |
|  | rule37         | -0.14864346 | week1 <= 1 & CSWAIT.T0 > 1    |                |
|  | rule17         | 0.14278100  | week1 > 0 & CSDEAL.T0 <= 3    |                |
|  | rule11         | -0.09730889 | week1 <= 0 & BSTENSE.T0 <= 2  |                |
|  | week1          | 0.03145116  | 0 <= week1 <= 7               |                |

The final ensemble consists of 7 terms. As expected, receiving TES is associated with lower substance use than TAU, as indicated by the negative coefficient of the confirmatory rule (`trt %in% 'TES'`). The `week1` variable obtained a positive coefficient, indicating that higher substance use in the first week of treatment is associated with higher substance use in the last week of treatment. The selected rules indicate that lower self-reported feelings of being scared (`BSSCARED.T0`) or tense (`BSTENSE.T0`) are associated with lower substance use in the last week of treatment. Higher self-reported coping skills (i.e., `CSWAIT.T0`: telling oneself that the urge to use substances will go away if one waits a while, and `CSDEAL.T0`: trying to remind oneself of the good things one

has accomplished) are associated with lower substance use during the last week of treatment.

Next, we request variable importances:

```
importance(drug_usage.ens)
```

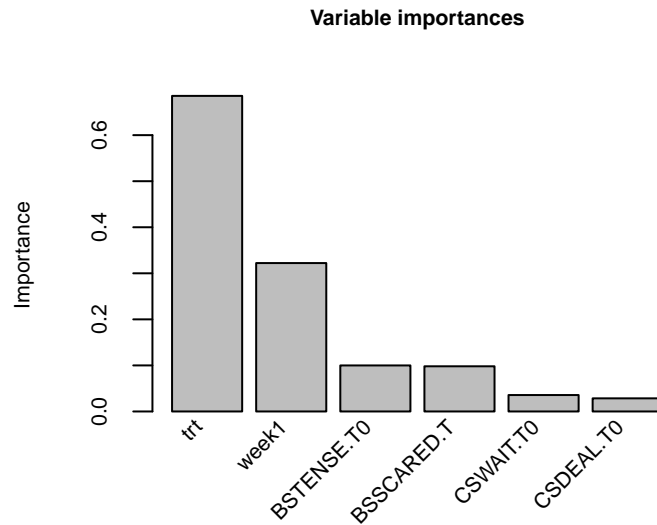

The plot indicates that the most important predictor of last-week substance use is the treatment indicator. First-week substance use is the next most important predictor. Self-reported symptoms of psychological distress (BSI) and coping skills (CSS) also contribute to the prediction of last-week substance use, but less strongly.

Again, to obtain an estimate of future prediction error, we apply function `cvpre()`:

```
cv.drug_usage <- cvpre(drug_usage.ens)
```

\$MSE

| MSE       | se        |
|-----------|-----------|
| 3.4963137 | 0.2918074 |

\$MAE

| MAE        | se         |
|------------|------------|
| 1.39536774 | 0.05699061 |

## Adjusting and Optimizing Parameters

In the examples above, we have mostly employed default settings of function `pre()`. However, `pre()` has several arguments for controlling the model-fitting procedure. By adjusting these settings, users can fine-tune accuracy and complexity of the final ensemble. The default settings of `pre()` represent the author’s choice of ‘sensible defaults’: settings that are expected to work well out-of-the-box, yielding relatively accurate and sparse ensembles.

However, sometimes users may prefer to use different settings, based on their subject-matter knowledge or specific requirements for application of the results. For example, maximum rule length may be specified based on a researcher’s prior knowledge about the order of interactions present in the data, or because rules defined by multiple conditions may be too complex or costly to evaluate in practical applications. Or, a researcher may be more interested in maximizing predictive accuracy than in minimizing complexity, vice versa.

Below, we discuss the parameters that can be adjusted to optimize accuracy, complexity and/or computation time. An extensive explanation of all arguments is provided in the help files, which can be accessed by typing `?`, followed by the function’s name. For example, we can access the help files for functions `pre()` and `importance()`, and the `predict` method, as follows:

```
?pre
?importance
?predict.pre
```

Below, we list the most important arguments of function `pre()`, their default values and how they most likely affect complexity, accuracy and/or computation time. We distinguish between ‘Model-Fitting’ and ‘Model-Selection’ parameters, where the former control how the initial ensemble of rules and/or linear functions is generated, and the latter control how the final ensemble is selected.

The set of parameter values that will provide optimal predictive accuracy may depend on the data problem at hand. Therefore, in the subsection “Tuning parameters for optimal predictive accuracy”, we will provide an example of fine-tuning the parameter values using cross validation, in order to maximize the expected predictive accuracy of the final ensemble.

## Model-Fitting Parameters

The following arguments can be passed to function `pre()` and determine how the initial ensemble of rules and/or linear terms is generated:

- **type**: This argument specifies the type of ensemble generated: **"both"** (the default) yields an initial ensemble of rules and linear terms. Alternatively, **"rules"** yields an initial ensemble of rules only and **"linear"** yields an ensemble of linear terms only.
- **ntrees**: Specifies the total number of trees to generate for rule induction. The default (500) corresponds to the default value of most random-forest algorithms. Lower values yield lower computation time and likely yield less complex, but also less accurate final ensembles. Higher values likely yield more complex ensembles and may increase the likelihood of overfitting.
- **sampfrac**: Specifies the fraction of randomly selected training observations used for fitting each tree. The default (.5) yields subsamples consisting of 50% of the training observations. Values between 0 and 1 yield sampling without replacement (i.e., subsampling). A value of 1 yields sampling with replacement (i.e., bootstrap sampling). Larger values may yield more complex final ensembles and somewhat higher computation times.
- **maxdepth**: Specifies the maximum number of conditions per rule. The default is 3, which yields rules consisting of at most three conditions. A value of 1 yields an additive model, with main effects only. Higher values allow for accommodating (higher-order) interactions, but also increase complexity of the final ensemble and may increase the likelihood of overfitting.
- **tree.unbiased**: Specifies whether unbiased recursive partitioning should be employed for rule generation. The default (**TRUE**) is to employ unbiased recursive partitioning as implemented in package **partykit** (Hothorn & Zeileis, 2015). If set to **FALSE**, the (biased) classification and regression trees algorithm (Breiman, Friedman, Olshen, & Stone, 1984) as implemented in package **rpart** (Therneau, Atkinson, & Ripley, 2017) will be employed. The latter reduces computation time, but will also yield more complex ensembles and possibly lower predictive accuracy.
- **learnrate**: Specifies the learning rate or boosting parameter applied in sequential tree induction. This parameter specifies the extent to which the response variable is ‘corrected’ for the predictions of earlier trees, prior to growing a new tree. A value of 0 yields no influence of earlier trees on later trees, while higher values yield increasing influence of earlier trees. Small, non-zero learning rates have been found to perform well in most problems (Friedman & Popescu, 2003), which is reflected in the default value

of .01. Higher values of the learning rate may yield less complex final ensembles.

- **mtry**: Specifies the number of predictor variables randomly selected as candidates for each split in each tree. The default (**Inf**) takes all potential predictors as candidates for each split. Specifying values  $> 0$  and  $< p$  (where  $p$  is the number of possible predictor variables) yields a random-forest style approach to rule induction and may decrease correlation between rules in the initial ensemble, which will reduce computation time and may improve predictive accuracy.
- **winsfrac**: Specifies the quantiles of the data distribution to be used for winsorizing (or censoring) linear terms, to reduce the effect of possible outliers. The default is .05, resulting in values lower than the .05 and higher than the .95 quantiles of a predictor variable's distribution to be set to the value of the .05 and .95 quantile, respectively. Lower values of **winsfrac** increase the effect of possible outliers. If set to 0, no winsorizing is performed.

## Model-Selection Parameter

The final ensemble is selected through penalized regression of the response variable on the rules and linear terms in the initial ensemble. Internally, package **pre** employs package **glmnet** (Friedman et al., 2010) to perform this penalized regression. To obtain the optimal value for the penalty parameter  $\lambda$ ,  $k$ -fold cross validation is used, with  $k = 10$ , by default. Parameter  $\lambda$  can take values between 0 and 1, with a value of 0 yielding an unpenalized solution and a value of 1 yielding an intercept-only solution.

The *optimal* value of  $\lambda$  is determined, based on one of two possible criteria that can be passed to the **penalty.par.val** argument: **"lambda.min"**, which returns a final ensemble selected with the  $\lambda$  value that yields the minimum cross-validated prediction error. By default, however, **pre()** employs **penalty.par.val = "lambda.1se"**, which returns a final ensemble selected with the  $\lambda$  value that yielded the least complex model, with a cross-validated prediction error within 1 standard error of the minimum. The **"lambda.1se"** criterion generally yields a  $\lambda$  value larger than that of the **"lambda.min"** criterion, in turn yielding less complex final ensembles, that may be less likely to overfit. Although the **"lambda.min"** criterion may yield slightly more accurate final ensembles than the default **lambda.1se** in some cases, it will almost always yield more complex final ensembles. The default criterion **"lambda.1se"** thus favors less complex ensembles, which are less likely to overfit.

The **penalty.par.val** argument can be passed to methods **summary**, **print**, **plot** and **coef**, and functions **importance()**, **singleplot()**, **pairplot()** and **cvpre()**.

## Tuning Parameters for Optimal Predictive Accuracy

Function `train()` from package **caret** (Kuhn, 2008) can be used to tune the parameters of a predictive method using cross validation, in order to optimize predictive accuracy of the final model. Here, we will use `train()` to assess which values for the `maxdepth`, `learnrate` and `penalty.par.val` parameters can be expected to yield highest predictive accuracy, for a PRE fitted to the data from Example 1 (predicting chronic depression). Then, if we want to fit a PRE which can be expected to provide optimal predictive accuracy, we should use those parameter values that provided the highest predictive accuracy, according to the cross-validation results.

Note that if the aim is to optimize predictive accuracy, the parameters of the fitting procedure should be tuned, prior to fitting and interpreting the PRE. In the current document, for instructional purposes, we have first fitted and interpreted a PRE using default settings in Example 1.

Package **pre** provides a model setup for `train()` by means of the `caret_pre_model` object, which contains all instructions necessary for `train()` to evaluate the effects of the parameters of function `pre()`. Below, we will construct a design matrix with parameter values, after which we will use `train()` to assess the cross-validated predictive accuracy for each combination of the parameter values specified.

If package **caret** was not installed yet, we first need to install it as follows:

```
install.packages("caret")
```

We load the package as follows:

```
library("caret")
```

The `caret_pre_model` object, which is part of package **pre**, is a list containing several elements:

```
names(caret_pre_model)
```

```
[1] "library"    "type"       "parameters" "grid"       "fit"        "predict"
[7] "prob"      "sort"       "loop"       "levels"     "tag"        "label"
[13] "predictors" "varImp"     "oob"        "notes"      "check"
```

The `grid` element is a function, which allows for creating a tuning grid: a factorial design matrix for all candidate tuning parameter values. As arguments to this function, we specify the parameters and values that we want to evaluate. Here, we will specify three values for `maxdepth`, three values for `learnrate`, and two values for `penalty.par.val`. The `grid()` function will automatically include the default values for the remaining parameter values that can be tuned:

```
tuneGrid <- caret_pre_model$grid(
  maxdepth = c(2, 3, 4), learnrate = c(0, .01, .1),
  penalty.par.val = c("lambda.min", "lambda.1se"))
head(tuneGrid)
```

|   | sampfrac | maxdepth | learnrate | mtry | use.grad | penalty.par.val |
|---|----------|----------|-----------|------|----------|-----------------|
| 1 | 0.5      | 2        | 0.00      | Inf  | TRUE     | lambda.min      |
| 2 | 0.5      | 3        | 0.00      | Inf  | TRUE     | lambda.min      |
| 3 | 0.5      | 4        | 0.00      | Inf  | TRUE     | lambda.min      |
| 4 | 0.5      | 2        | 0.01      | Inf  | TRUE     | lambda.min      |
| 5 | 0.5      | 3        | 0.01      | Inf  | TRUE     | lambda.min      |
| 6 | 0.5      | 4        | 0.01      | Inf  | TRUE     | lambda.min      |

Next, we separate the data into the response (y) and potential predictor variables (x):

```
y <- depression$dep
x <- depression[, -1]
```

We can now apply function `train()`, by specifying the predictor and response variables, `caret_pre_model` as the method and `tuneGrid` as the tuning grid. We specify the `trControl` argument, in order to employ cross validation to estimate predictive accuracy of the fitted models (by default, ten folds will be used). We specify the `family` argument, which will be passed to function `pre()` to clarify that the response is a binary factor. As cross validation depends on random sampling of the training observations, we first set the random seed, to allow for later replication of the results:

```
set.seed(4)
fit <- train(x = x, y = y, method = caret_pre_model, tuneGrid = tuneGrid,
  trControl = trainControl("cv"), family = "binomial")
```

Note that the call to `train()` will take quite some time to run, as it fits a PRE for every combination of the tuning parameters, in each of the ten folds.

When the computations are finished, we can print the results using the `print` method. Here, we also specify the `showSD` argument, in order to have the standard deviations over the ten folds included in the results, and we specify the `digits` argument, to have the accuracy estimates rounded to three digits. We specify the `selectCol` argument, so the set of parameters that yielded highest predictive accuracy will be indicated with an asterisk:

```
print(fit, showSD = TRUE, digits = 3, selectCol = TRUE)
```

Prediction Rule Ensembles

```

682 samples
20 predictor
2 classes: 'No', 'Yes'

```

No pre-processing

Resampling: Cross-Validated (10 fold)

Summary of sample sizes: 613, 614, 613, 613, 614, 614, ...

Resampling results across tuning parameters (values below are 'mean (sd)'):

| maxdepth | learnrate | penalty.par.val | Accuracy       | Kappa          | Selected |
|----------|-----------|-----------------|----------------|----------------|----------|
| 2        | 0.00      | lambda.min      | 0.585 (0.0606) | 0.170 (0.1214) |          |
| 2        | 0.00      | lambda.1se      | 0.596 (0.0643) | 0.193 (0.1282) |          |
| 2        | 0.01      | lambda.min      | 0.588 (0.0821) | 0.175 (0.1643) |          |
| 2        | 0.01      | lambda.1se      | 0.589 (0.0646) | 0.179 (0.1291) |          |
| 2        | 0.10      | lambda.min      | 0.582 (0.0770) | 0.164 (0.1537) |          |
| 2        | 0.10      | lambda.1se      | 0.600 (0.0808) | 0.201 (0.1617) |          |
| 3        | 0.00      | lambda.min      | 0.589 (0.0523) | 0.178 (0.1044) |          |
| 3        | 0.00      | lambda.1se      | 0.595 (0.0739) | 0.190 (0.1479) |          |
| 3        | 0.01      | lambda.min      | 0.585 (0.0617) | 0.169 (0.1234) |          |
| 3        | 0.01      | lambda.1se      | 0.589 (0.0764) | 0.178 (0.1530) |          |
| 3        | 0.10      | lambda.min      | 0.591 (0.0585) | 0.181 (0.1167) |          |
| 3        | 0.10      | lambda.1se      | 0.598 (0.0761) | 0.196 (0.1528) |          |
| 4        | 0.00      | lambda.min      | 0.580 (0.0537) | 0.161 (0.1074) |          |
| 4        | 0.00      | lambda.1se      | 0.599 (0.0718) | 0.199 (0.1432) |          |
| 4        | 0.01      | lambda.min      | 0.579 (0.0425) | 0.158 (0.0849) |          |
| 4        | 0.01      | lambda.1se      | 0.602 (0.0733) | 0.205 (0.1468) |          |
| 4        | 0.10      | lambda.min      | 0.601 (0.0639) | 0.202 (0.1280) |          |
| 4        | 0.10      | lambda.1se      | 0.614 (0.0688) | 0.229 (0.1373) | *        |

Tuning parameter 'sampfrac' was held constant at a value of 0.5

Tuning

parameter 'mtry' was held constant at a value of Inf

Tuning parameter

'use.grad' was held constant at a value of TRUE

Accuracy was used to select the optimal model using the largest value.

The final values used for the model were sampfrac = 0.5, maxdepth = 4, learnrate = 0.1, mtry = Inf, use.grad = TRUE and penalty.par.val = lambda.1se.

The resulting table lists the means of the accuracy estimates over the 10 cross-validation folds, with standard deviations in parentheses. Two measures of predictive accuracy are provided: **Accuracy** represents the proportion classified correctly, **Kappa** represents the same proportion, but corrected for the base rate. A Kappa value of 1 indicates perfect predictive accuracy, a value of 0 indicates predictive accuracy no better

than chance.

Highest accuracy was obtained with a maximum rule length of 4, a learning rate of 0.1, and a penalty parameter value of `lambda.1se`, yielding an accuracy of 0.61 ( $SD = 0.069$ ). The default settings (`maxdepth = 3`, `learnrate = .01`, `penalty.par.val = "lambda.1se"`) yielded an accuracy of 0.589 ( $SD = 0.076$ ). These standard deviations can be interpreted as standard errors of the accuracy estimates. Thus, for this dataset, the improvement that may be obtained by using the optimal parameter settings determined through cross validation, appears small: the difference in performance between the optimal and default settings is less than one standard error.

Still, we could prefer to employ these tuned or optimized values, instead of the default settings. For example, because our sole aim is to optimize predictive accuracy, or because the lower values of `maxdepth` and `learnrate` may provide a less complex ensemble. In that case, we would fit our PRE as follows (further results omitted):

```
depression.ens <- pre(dep ~ ., data = depression, maxdepth = 2,  
                     learnrate = .1, family = "binomial")
```

## References

- Breiman, L., Friedman, J., Olshen, R., & Stone, C. (1984). *Classification and regression trees*. New York: Wadsworth.
- Fokkema, M. (n.d.). Fitting prediction rule ensembles with R package pre. *Journal of Statistical Software*. Retrieved from <https://arxiv.org/abs/1707.07149>
- Friedman, J., Hastie, T., & Tibshirani, R. (2010). Regularization paths for generalized linear models via coordinate descent. *Journal of Statistical Software*, 33(1), 1–22. Retrieved from <http://www.jstatsoft.org/v33/i01/>
- Friedman, J., & Popescu, B. E. (2003). Importance sampled learning ensembles. Technical Report, Stanford University. Retrieved from <http://www-stat.stanford.edu/~jhf/ftp/isle.pdf>
- Hothorn, T., & Zeileis, A. (2015). partykit: A modular toolkit for recursive partytioning in R. *Journal of Machine Learning Research*, 16, 3905–3909.
- Kuhn, M. (2008). Building Predictive Models in R Using the caret Package. *Journal of Statistical Software*, 28(5), 1–26. doi:10.18637/jss.v028.i05

R Core Team. (2019). *R: A language and environment for statistical computing*. Vienna, Austria: R Foundation for Statistical Computing. Retrieved from <https://www.R-project.org/>

Therneau, T., Atkinson, B., & Ripley, B. (2017). *rpart: Recursive partitioning and regression trees*. Retrieved from <https://CRAN.R-project.org/package=rpart>

Torfs, P., & Brauer, C. (2014). A (very) short introduction to R. Tutorial, Hydrology and Quantitative Water Management Group, Wageningen University, The Netherlands. Retrieved from <https://cran.r-project.org/doc/contrib/Torfs+Brauer-Short-R-Intro.pdf>
